# Supplementary material for: Fraction of clogging configurations sampled by granular hopper flow
Source: arXiv:1410.0933 source file (2015-05-05)
Supplement: Supplementary file 1 [file CloggingSupplement.pdf]

# Supplemental Material for “Fraction of clogging configurations sampled by granular hopper flow[1]”

C. C. Thomas and D. J. Durian
*University of Pennsylvania, Department of Physics & Astronomy*

(December 17, 2014)

We construct a model of clogging in which there is the same history-independent probability to clog at each step in a sequence of constant time increments, but where there is a minimum discharge event size. It compares well with data from Ref. [2] for how the standard deviation of discharge masses $\sigma_m$ falls below the average $\langle m \rangle$ for small events. The results support findings in the main text for $F = \rho A\ell/\langle m \rangle$ as the fraction of clogging configurations and also for $\ell = 0.75d$ as the sampling length [1]. We also present variations of the model, and compare to data from Ref. [3].

## 1 Clogging as a discrete Poisson process

The distribution of discharge events may be computed exactly, assuming only that in each sampling time step $\tau_0$ there is the same constant probability $\alpha$ for the system to clog. The value of $\alpha$, as well as the discharge speed $v$, will vary with the area $A = \pi(D/2)^2$ of the hole and with the nature of the grains. But for any given $\alpha$ the probability to flow for $n$ sampling times, and then clog at the next sampling time, is equal to the product $(1-\alpha)^n\alpha$ of probabilities at each step. This is automatically normalized, $\sum_{n=0}^{\infty}(1-\alpha)^n\alpha = 1$, but only if the sum starts at $n = 0$. However, experimentalists do not count $n = 0$ “null” events where no mass is discharged. Flow events are initiated by external impulses that, by design, are large enough to cause measurable discharge. Therefore we restrict $n$ to be $1, 2, 3, \ldots$, and introduce a normalization factor. Then

$$p(n) = (1-\alpha)^{n-1}\alpha \tag{1}$$

is the probability to flow for time $\tau = n\tau_0$ and to discharge mass $m = \rho A v\tau = \rho A\ell n$, where $\rho$ is the mass density of the bulk granular medium and $\ell = v\tau_0$ is the sampling length as in the main text. In this model, the smallest allowed discharge event has mass $\rho A\ell$, which corresponds to about a monolayer of grains spanning the hole if $\ell$ is on the order of the grain diameter $d$. This is reminiscent of the classic “free-fall

arch" rationalization of the Beverloo discharge rate equation, recently discussed in Ref. [4], where a succession of unstable monolayer arches form, then break, then free-fall. Here we picture that a new monolayer appears once per sampling time, and that with probability $\alpha$ it is actually stable. The cumulative distribution for Eq. (1) is

$$c(n) = \sum_{n'=1}^{n} p(n') = 1 - (1-\alpha)^n. \tag{2}$$

Note that for small $\alpha$ the distribution of flow durations becomes a continuous exponential: $p(\tau) = \left[p(n)\frac{\mathrm{d}n}{\mathrm{d}\tau}\right]_{n=\tau/\tau_0} = \exp(-\tau/\langle\tau\rangle)/\langle\tau\rangle$ where $\langle\tau\rangle$ is defined as $\tau_0/\alpha$ and is equal to the average flow duration.

For geometrical distributions like Eq. (1) it is straightforward to compute the moments $\langle n^m\rangle = \sum_{n=1}^{\infty} n^m p(n)$, exactly, for any $\alpha$. The first two moments and the standard deviation of $n$, and hence of the discharge masses $m = \rho A\ell n$, are

$$\langle n\rangle = \frac{\langle m\rangle}{\rho A\ell} = \frac{1}{\alpha}, \tag{3}$$

$$\langle n^2\rangle = \frac{\langle m^2\rangle}{(\rho A\ell)^2} = \frac{2}{\alpha^2} - \frac{1}{\alpha}, \tag{4}$$

$$\sigma_n = \frac{\sigma_m}{\rho A\ell} = \sqrt{\frac{1}{\alpha^2} - \frac{1}{\alpha}}. \tag{5}$$

Comparison of Eq. (3) with Eq. (1) of the main text, $F = \rho A\ell/\langle m\rangle$, shows that the probability $\alpha$ to clog in each sampling time is equivalent to the fraction $F$ of clogging configurations. We may now combine Eqs. (3,5) to eliminate $\alpha$ and reveal the expected connection between $\sigma_m$ and $\langle m\rangle$ if clogging is a discrete Poisson process:

$$\sigma_m = \sqrt{\langle m\rangle\left(\langle m\rangle - \rho A\ell\right)}, \tag{6}$$

$$\frac{\sigma_m}{\rho A d} = \sqrt{\frac{\langle m\rangle}{\rho A d}\left(\frac{\langle m\rangle}{\rho A d} - \frac{\ell}{d}\right)}. \tag{7}$$

Note that $\sigma_m \to \langle m\rangle$ in the limit of small $\alpha$ and hence of large $\langle m\rangle$, where the distributions are exponential. Eq. (7) is made dimensionless by $\rho A d$ as the characteristic mass controlled by the experimentalist. If $\ell/d$ is thought to be a constant independent of hole size, then data for $\sigma_m/(\rho A d)$ may be plotted versus $\langle m\rangle/(\rho A d)$ and compared with $y = \sqrt{x(x-\ell/d)}$ to test the model and to determine the value of $\ell/d$.

## 1.1 Comparison with $\sigma_m$ data

We now compare the above predictions with data from Ref. [2] on the standard deviation of the discharge event mass distribution for tilted hoppers. For a given tilt, the average mass $\langle m\rangle$ and the standard deviation $\sigma_m$ both increase with hole size.

These quantities are divided by $\rho A d$ and are plotted parametrically in Fig. 1. The data spanabout four orders of magnitude, and are scattered around $\sigma_m = \langle m \rangle$ for $\langle m \rangle/(\rho A d)$ greater than about 10. Thus, large events are consistent with a continuous exponential distribution. For smaller events, $\sigma_m$ falls noticeably below $\langle m \rangle$; however, just such behavior is predicted by the above model of clogging as a discrete Poisson process. For direct comparison, Eq. (7) is plotted in Fig. 1, using $\ell/d = 0.75 \pm 0.20$ as found in the main text by requiring $F$ to extrapolate to 1 as the hole area decreases to the grain cross sectional area. This curve is quite consistent with the data, though the data appear to deviate from $y = x$ sooner than the model. Alternatively, fitting Eq. (7) to the data gives $\ell/d = 0.73 \pm 0.08$ (the uncertainty also reflects inclusion or exclusion of smallest data point, which could be an outlier). The good general agreement seen in Fig. 1, both for the form of $\sigma_m$ versus $\langle m \rangle$ and for the value of $\ell/d$, supports the assumptions and findings in the main text.

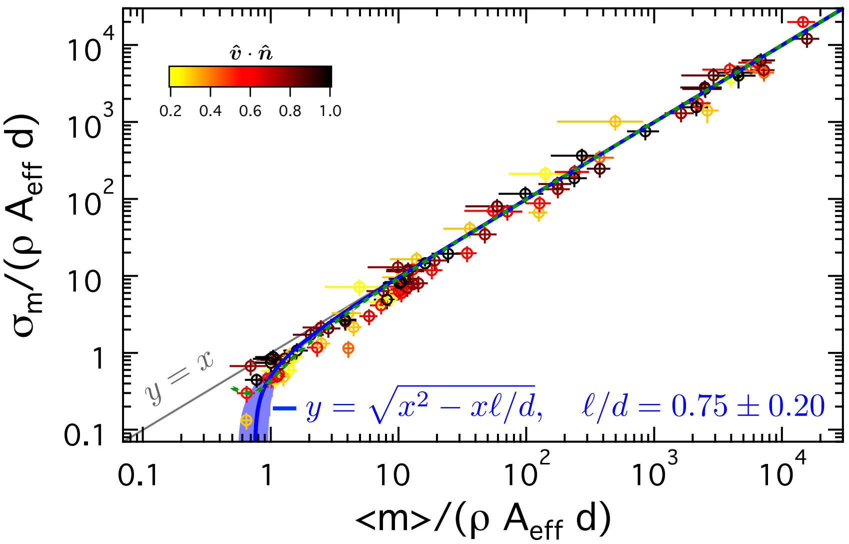


Figure 1: Standard deviation of mass versus average mass for $d = 2$ mm diameter glass spheres, of bulk density $\rho = 1.62$ g/cm$^3$, discharged from circular holes with effective area $A_{\text{eff}} = A\hat{v} \cdot \hat{n}$. Data are from Fig. 3a of Ref. [2]. The gray line $y = x$ is the expectation for an exponential distribution. The blue curve and shaded region are Eq. (7) with $\ell/d = 0.75 \pm 0.20$ taken from the main text. The green dashed curve represents Eq. (10) with $\ell/d = 0.6$, $\overline{n}_o = 1.6$, $\sigma_n = 0.7$.

## 1.2 Generalization

One may take $p(n) = (1-\alpha)^{n-n_o}\alpha$ with $n = n_o, n_o+1, n_o+2, \ldots$ as a more general model of clogging, where $n_o$ is number of sample times for the smallest allowed discharge event. Above we use $n_o = 1$, but other values could be appropriate when large or variable impulses are used to start the flow events. This gives a cumulative distribution of

$c(n) = 1 - (1-\alpha)^{n-n_o+1}$. The first two moments are

$$\langle n \rangle = \frac{\langle m \rangle}{\rho A \ell} = \frac{1}{\alpha} - 1 + n_o, \tag{8}$$

$$\langle n^2 \rangle = \frac{\langle m^2 \rangle}{(\rho A \ell)^2} = \left(\frac{2}{\alpha^2} - \frac{3}{\alpha} + 1\right) + 2\left(\frac{1}{\alpha} - 1\right) n_o + {n_o}^2. \tag{9}$$

To average these over an arbitrary distribution of $n_o$, with average $\overline{n}_o$ and standard deviation $\sigma_{n_o}$, we substitute $n_o \to \overline{n}_o$ and ${n_o}^2 \to \overline{{n_o}^2} = ({\overline{n}_o}^2 + {\sigma_{n_o}}^2)$. Using $m = \rho A \ell n$ and eliminating $\alpha$, as above, the standard deviation of discharge masses is found as

$$\frac{\sigma_m}{\rho A d} = \sqrt{\left[\frac{\langle m \rangle}{\rho A d} - (\overline{n}_o - 1)\frac{\ell}{d}\right]\left[\frac{\langle m \rangle}{\rho A d} - \overline{n}_o \frac{\ell}{d}\right] + \left(\sigma_{n_o}\frac{\ell}{d}\right)^2}\,. \tag{10}$$

This generalizes upon Eq. (7) for non-integer $\overline{n}_o > 1$ and for $\sigma_{n_o} > 0$. Note that a variation of $\ell/d$ is nearly cancelled by a reciprocal variation of $\overline{n}_o$ and $\sigma_{n_o}$. Therefore in Fig. 1 we show a fit where $\ell/d = 0.6$ is fixed toward the lower end of the range found in the main text and the other two parameters are optimized. This gives reasonable values of $\overline{n}_o = 1.6 \pm 0.3$ and $\sigma_{n_o} = 0.7 \pm 0.2$, and good agreement with the data.

The generalized model may also explain the peaked shape of the event distribution data in Ref. [3]. There, the probability functions started from a minimum event size, increased steeply to a maximum, and then decayed exponentially with a longer decay constant. This was modeled by a transient, where steady-flow is achieved only after some delay. Here, transients are not in flow speed but in disallowing clogging at less than some numbers $n_o > 1$ of sampling times. The mode of the averaged distribution is then roughly $\overline{n}_o$. In terms of mass and number of grains, this gives

$$m_{\text{mode}} \approx \rho A \ell \overline{n}_o, \tag{11}$$

$$S_{\text{mode}} = \frac{m_{\text{mode}}}{m_{\text{grain}}} \approx \frac{3\phi}{2}\left(\frac{D}{d}\right)^2 \left(\frac{\ell}{d}\right)\overline{n}_o, \tag{12}$$

where $\phi$ is the volume fraction of grains in the packing [5]. Indeed, the inset of Fig. 3a of Ref. [3] shows that the mode grows quadratically with hole size. Taking $\phi = 0.64$ and $\ell/d = 0.75$, the mode data correspond roughly to Eq. (12) with $\overline{n}_o \approx 2$. One could imagine a detailed analysis where $\ell/d$ and the full distribution of $n_o$ are obtained from experimental event distribution data.

# 2 Clogging as a continuous nearly-Poisson process

The deviation of data from $\sigma_m = \langle m \rangle$ for small events is accounted for in the models both by discretization and by the existence of a smallest allowed discharge mass. In

attempt to disentangle these effects, we now consider two *ad-hoc* flow distributions that are continuous. The first is zero below a sampling time $\tau_0$, and is exponential otherwise:

$$p(t) = \begin{cases} 0 & t < \tau_0, \\ Re^{-R(t-\tau_0)} & t > \tau_0, \end{cases} \tag{13}$$

where $R$ is a rate constant independent of the sampling time. The first two moments are $\langle t \rangle = (1/R) + \tau_0$ and $\langle t^2 \rangle = (2/R^2) + (2/R)\tau_0 + {\tau_0}^2$. To average over an arbitrary distribution of sampling times, we take $\tau_0 \to \overline{\tau}_0$ and ${\tau_0}^2 \to \overline{{\tau_0}^2} = ({\overline{\tau}_0}^2 + {\sigma_{\tau_0}}^2)$. Eliminating $R$, using $m = \rho A v t$ and $\langle \ell \rangle = v\overline{\tau}_0$, then dividing through by $\rho A d$, gives the standard deviation of discharge masses as

$$\frac{\sigma_m}{\rho A d} = \sqrt{\left(\frac{\langle m \rangle}{\rho A d} - \frac{\langle \ell \rangle}{d}\right)^2 + \left(\frac{\sigma_\ell}{d}\right)^2}. \tag{14}$$

The behavior is $\sigma_m = \langle m \rangle$ for large $\langle m \rangle$, and $\sigma_m < \langle m \rangle$ for smaller discharges. Similar to the discrete model, the smallest hole size corresponds to $\langle m \rangle = \rho A \langle \ell \rangle$. There, $\sigma_m$ is at a minimum that is non-zero for $\sigma_\ell > 0$. In Fig. 2 we fit to to Eq. (14), which gives $\langle \ell/d \rangle = 0.7 \pm 0.2$ and $\sigma_\ell/d = 0.3 \pm 0.2$ in reasonable agreement with the data.

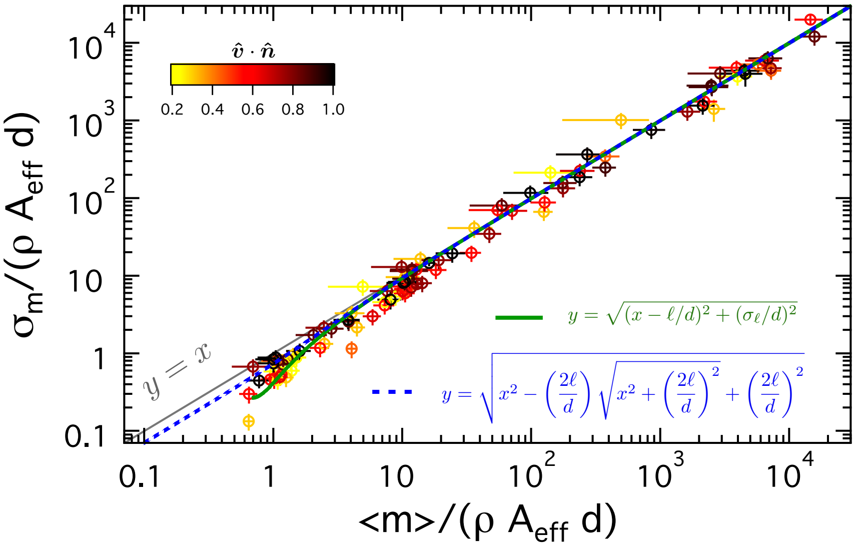


Figure 2: Same data as Fig. 1 but now comparing with two models that have a continuous distribution of discharge event sizes. The solid green curve is Eq. (14) with fit values $\ell/d = 0.7 \pm 0.2$ and $\sigma_\ell/d = 0.3 \pm 0.2$. The dashed blue curve is Eq. (16) with $\ell/d = 0.75$ as in the main text.

For contrast, the following probability function smoothly suppresses small flow events but has no cutoff:

$$p(t) \propto \left(1 - e^{-t/\tau_0}\right) e^{-Rt}. \tag{15}$$

The first two moments may be computed, and lead to a standard deviation of discharge masses of

$$\frac{\sigma_m}{\rho A d} = \sqrt{\left(\frac{\langle m\rangle}{\rho A d}\right)^2 - \left(\frac{2\ell}{d}\right)\sqrt{\left(\frac{\langle m\rangle}{\rho A d}\right)^2 + \left(\frac{2\ell}{d}\right)^2} + \left(\frac{2\ell}{d}\right)^2}, \tag{16}$$

The behavior is also $\sigma_m = \langle m\rangle$ for large $\langle m\rangle$, and $\sigma_m < \langle m\rangle$ for smaller discharges. But now, there is no minimum discharge mass and $\sigma_m$ vanishes smoothly as $\langle m\rangle$ goes to zero. This form is rather insensitive to the value of $\ell/d$. So in Fig. 2 we simply plot Eq. (16) with the value $\ell/d = 0.75$ from the main text. The agreement is not bad, but for the smallest $\langle m\rangle$ the data do deviate a little more from $\sigma_m = \langle m\rangle$ than Eq. (16).

Our impression from these comparisons is that the existence and treatment of the minimum discharge event size has more influence on the form of $\sigma_m$ versus $\langle m\rangle$ than on whether the discharge distribution is treated as continuous or discrete. We also see that the sampling length reported in the main text, $\ell = (0.75 \pm 0.20)d$, is consistent with all of the Poisson process models.

# 3 Acknowledgments

This work was supported by the NSF through Grant Number DMR-1305199.

# References

[1] C. C. Thomas and D. J. Durian, "Fraction of clogging configurations sampled by granular hopper flow," arXiv:1410.0933.

[2] C. C. Thomas and D. J. Durian, "Geometry dependence of the clogging transition in tilted hoppers," Phys. Rev. E **87**, 052201 (2013).

[3] I. Zuriguel, A. Garcimartín, D. Maza, L. A. Pugnaloni, and J. M. Pastor, "Jamming during the discharge of granular matter from a silo," Phys. Rev. E **71**, 051303 (2005).

[4] A. Janda, I. Zuriguel, D. Maza, "Flow rate of particles through apertures obtained from self-similar density and velocity profiles," Phys. Rev. Lett. **108**, 248001 (2012).

[5] Similarly the minimum event size is $S_{\rm min} = \rho A\ell/m_{\rm grain} = (3\phi/2)(D/d)^2(\ell/d)$. It is one grain if $\ell/d = (d/D)^2$, assuming a packing fraction of $\phi = 2/3$. One could imagine $\ell/d$ crossing over from such behavior at small holes to constant $\ell/d = 0.75$ at large holes, where even the smallest impulse causes many grains to discharge.
